# Supplementary material for: A singlet triplet hole spin qubit in planar Ge
Source: arXiv:2011.13755 ancillary file (2021-04-07)
Supplement: Supplementary file 1 [file Supplementary.pdf]

# Supplementary Information: A singlet triplet hole spin qubit in planar Ge

Daniel Jirovec[1], Andrea Hofmann[1], Andrea Ballabio[2], Philipp M. Mutter[3],

Giulio Tavani[2], Marc Botifoll[4], Alessandro Crippa[1], Josip Kukucka[1],

Oliver Sagi[1], Frederico Martins[1], Jaime Saez-Mollejo[1], Ivan Prieto[1],

Maksim Borovkov[1], Jordi Arbiol[4,5], Daniel Chrastina[2], Giovanni Isella[2], Georgios Katsaros[1]

[1]Institute of Science and Technology Austria, Am Campus 1, 3400 Klosterneuburg, Austria
[2]L-NESS, Physics Department, Politecnico di Milano, via Anzani 42, 22100, Como, Italy
[3]Department of Physics, University of Konstanz, D-78457 Konstanz, Germany
[4]Catalan Institute of Nanoscience and Nanotechnology (ICN2), CSIC and BIST, Campus UAB, Bellaterra, Barcelona, Catalonia, Spain
[5]ICREA, Passeig de Lluís Companys 23, 08010 Barcelona, Catalonia, Spain

April 7, 2021

## 1 The Model

We assume the heavy-hole double quantum dot (DQD) system to be in the (1,1)-(2,0) regime such that the (0,2) charge configuration and all triplet states consisting of a doubly occupied dot are split off energetically and may be neglected. Hence, the Hilbert space under consideration is spanned by the (2,0) singlet $|S_{20}\rangle$, the (1,1) singlet $|S\rangle$ and the three (1,1) triplet states $|T_{0,\pm}\rangle$. The two singlet states are detuned by an amount $\epsilon = U - \tilde{\epsilon}$, where $U$ is the charging energy and $\tilde{\epsilon}$ is the energy difference between the two dots in the one-particle picture. At positive detunings, $\epsilon > 0$, the (1,1) singlet is energetically favourable. The parts of the Hamiltonian describing the basic DQD system and the spin-orbit interaction (SOI) read, respectively,

$$H_0 = \epsilon|S_{20}\rangle\langle S_{20}| + \sqrt{2}t_c \left(|S_{20}\rangle\langle S| + |S\rangle\langle S_{20}|\right), \tag{1}$$

$$H_{\mathrm{SO}} = t_{\mathrm{SO}} \sum_{\pm} \left(|S_{20}\rangle\langle T_\pm| + |T_\pm\rangle\langle S_{20}|\right), \tag{2}$$

where $t_c$ is the one-particle tunneling element and $t_{\mathrm{SO}}$ parametrizes spin-flip tunneling events induced by the SOI. The unpolarized triplet does not appear in Eq. (2) as the SOI of Ge hole states in similar systems has been found to couple the singlet in the (2,0) configuration to the polarized triplets only [1].

When applying an out-of-plane magnetic field of magnitude $B$ and taking into account site-dependent $g$-tensors, the Hamiltonian of the system contains a Zeeman term of the form [2],

$$H_Z = \frac{\mu_B B}{2} \sum_{d\in\{L,R\}} g_d \sigma_z^d, \tag{3}$$

where $\sigma_z^d$ is the Pauli matrix along the quantization axis and $g_d$ labels the out-of-plane $g$-factor in the left ($d = L$) and right ($d = R$) dot.

In the presence of a finite tunnel coupling $t_c$ the singlets form hybridized states according to Eq. (1),

$$\begin{aligned} |S_G\rangle &= \cos\frac{\Omega}{2}|S\rangle + \sin\frac{\Omega}{2}|S_{20}\rangle, \\ |S_E\rangle &= \cos\frac{\Omega}{2}|S_{20}\rangle - \sin\frac{\Omega}{2}|S\rangle, \end{aligned} \tag{4}$$

with the mixing angle $\Omega = -\arctan\left(\frac{2\sqrt{2}t_c}{\epsilon}\right)$. Consequently, the total Hamiltonian $H = H_0 + H_{\mathrm{SO}} + H_Z$ reads in the basis $\{|S_E\rangle, |S_G\rangle, |T_+\rangle, |T_0\rangle, |T_-\rangle\}$,

$$H = \begin{pmatrix} \frac{\epsilon}{2} + \sqrt{\frac{\epsilon^2}{4} + 2t_c^2} & 0 & t_{\mathrm{SO}}\cos\frac{\Omega}{2} & -\frac{\Delta g \mu_B B}{2}\sin\frac{\Omega}{2} & t_{\mathrm{SO}}\cos\frac{\Omega}{2} \\ 0 & \frac{\epsilon}{2} - \sqrt{\frac{\epsilon^2}{4} + 2t_c^2} & t_{\mathrm{SO}}\sin\frac{\Omega}{2} & \frac{\Delta g \mu_B B}{2}\cos\frac{\Omega}{2} & t_{\mathrm{SO}}\sin\frac{\Omega}{2} \\ t_{\mathrm{SO}}\cos\frac{\Omega}{2} & t_{\mathrm{SO}}\sin\frac{\Omega}{2} & \frac{\Sigma g \mu_B B}{2} & 0 & 0 \\ -\frac{\Delta g \mu_B B}{2}\sin\frac{\Omega}{2} & \frac{\Delta g \mu_B B}{2}\cos\frac{\Omega}{2} & 0 & 0 & 0 \\ t_{\mathrm{SO}}\cos\frac{\Omega}{2} & t_{\mathrm{SO}}\sin\frac{\Omega}{2} & 0 & 0 & -\frac{\Sigma g \mu_B B}{2} \end{pmatrix}, \tag{5}$$

where $\Sigma g$ ($\Delta g$) denotes the sum (difference) of out-of-plane $g$-factors. The energy spectrum resulting from this Hamiltonian is displayed in Fig. 2c of the main text. In the regime $\frac{t_c}{\epsilon} \ll 1$, one has $\sin\frac{\Omega}{2} \approx 0$ and $\cos\frac{\Omega}{2} \approx 1$, allowing us to work in the approximately decoupled subspace spanned by the ground state singlet $|S_G\rangle$ and the unpolarized triplet $|T_0\rangle$. Defining the exchange energy,

$$J(\epsilon) := \sqrt{\frac{\epsilon^2}{4} + 2t_c^2} - \frac{\epsilon}{2} > 0, \tag{6}$$

the effective qubit Hamiltonian takes on the compact form displayed in Eq. 1 of the main text.

### 1.1 Simulations

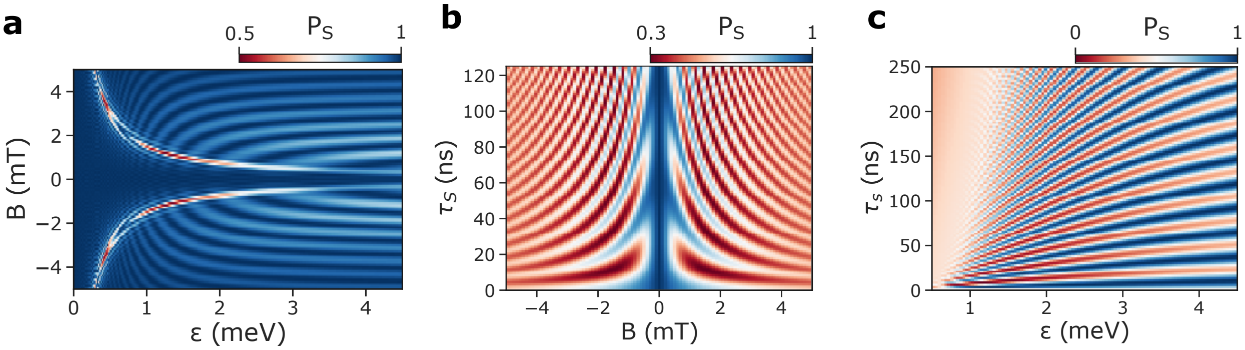


Figure S1: Simulations performed in Qutip. The time evolution is calculated with a master equation solver. a) Funnel simulation with the values for $J$, $\Sigma g$, $\Delta g$ extracted from the measurements of the main text (Figs. 3 and 4) and $t_{SO} = 100\,\mathrm{neV}$. All the main features of the funnel in Fig.2e are visible. b) Simulation of $S - T_0$ oscillations with the experimental values of Fig. 3c. We model the reduction in visibility with magnetic field as $V = V_0 \exp\{-B/B_0\}$ with $B_0 = 2.5\,\mathrm{mT}$. c) Simulation of the exchange oscillation experiment in Fig.4c. The decay is modelled with collapse operators $\sigma_Z$ with a rate proportional to $\frac{dJ}{d\epsilon}$ as in Fig. 4i of the main text.

## 2 Setup

All the measurements are performed in a dilution refrigerator from Leiden Cryogenics with a base temperature of 25 mK and an electron temperature of roughly 100 mK. The DC voltages are provided by a Delft IVVI electronics rack, the voltage pulses are generated by a Zurich instruments HDAWG and the reflectometry signal is generated and demodulated by a Zurich instruments UHFLI. The wiring of the high frequency lines is depicted in Fig. S2 with the attenuation at each fridge plate. A 0 dB attenuator serves as a thermal anchor and thermalizes the electrons to the temperature of that stage. The values of attenuation are chosen to maximize the noise suppression while not exceeding the cooling power and attenuating the signal too much. The sample is mounted on a printed circuit board designed in-house and hosts RC LP-filters for the DC lines (cutoff frequency 1.6 kHz ), bias Tees for the high frequency lines (cutoff at 1.8 MHz) and the LC-resonator for reflectometry (L = 2.2 µH, $C = C_p \approx 1\,\mathrm{pF}$). The reflectometry signal is passed through a directional coupler (Mini circuits ZFDC-20-50-s+), and is amplified on its way back by a low temperature CITLF amplifier (Cosmic Microwave Technologies).

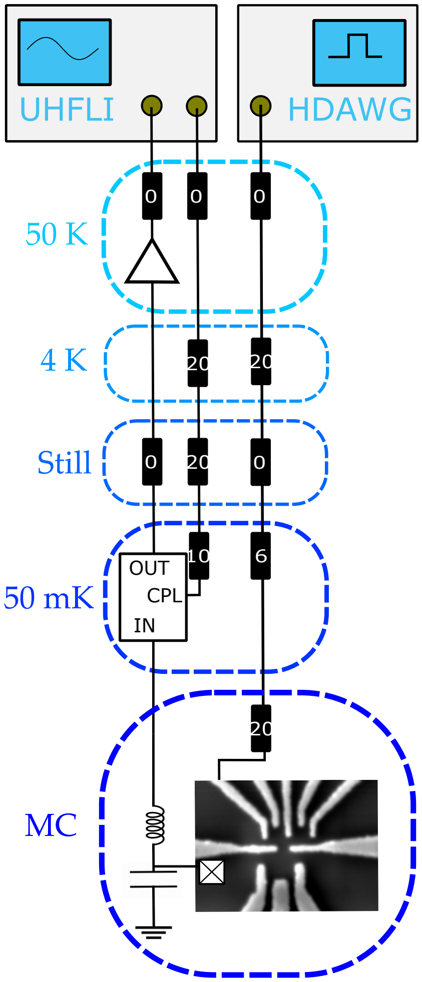


Figure S2: Setup. Attenuators at each stage of the cooling process ensure low electron temperature while maintaining a sizeable signal. The UHFLI provides and demodulates the microwave reflectometry tone. The HDAWG generates the fast pulses for qubit manipulation.

# 3 Structural characterizations

## 3.1 TEM

Structural characterization was performed on the samples by means of aberration corrected (AC) high-angle annular dark-field scanning transmission electron microscopy (HAADF-STEM) in a probe corrected Titan FEI microscope operated at 300 kV. The cross-section lamellae have been obtained by Focused Ion Beam in a FEI HELIOS 600 FIB. Electron energy loss spectra (EELS) were obtained in a GATAN Quantum spectrometer coupled to a field emission gun FEI F20 microscope operated at 200 kV. In order to map the atomic lattice dilatation and calculate the strain present at the QW, we have used geometric phase analyses (GPA), developed by Hytch[3;4].

## 3.2 XRD

High-resolution X-ray diffraction (HR-XRD) was carried out using Cu K$\alpha$1 radiation in a PANalytical X'Pert Pro MRD system equipped with a hydrid mirror and two-bounce Ge(220) monochromator on the primary beam, precision Euler cradle, and three-bounce analyser crystal in front of the detector. An $\omega$–$2\theta$ scan through the (004) Bragg peak (Fig. S3) was dynamically simulated[5] to confirm that the Ge QW is 18 nm thick, as shown in the profile in the inset.

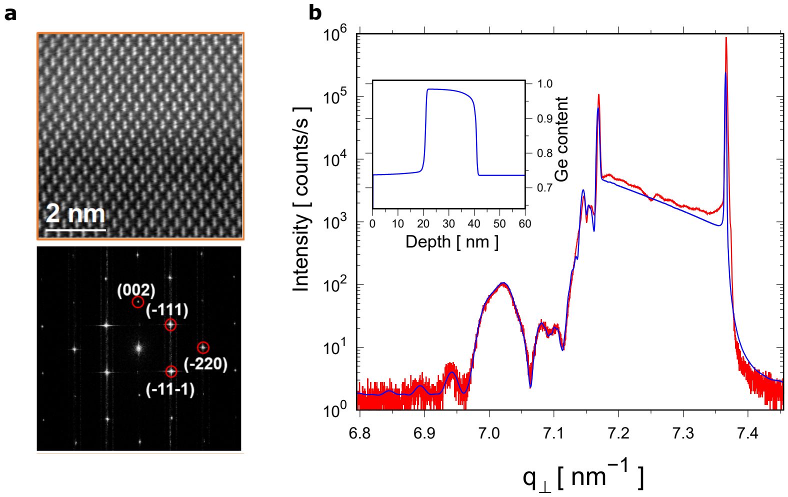


Figure S3: a)Atomic resolution aberration corrected (AC) high-angle annular dark-field scanning transmission electron microscopy (HAADF-STEM) image. We observe in-plane lattice matching between the ($\bar{2}$20) vertical planes that can be seen in the upper image (zoom in on bottom interface of Fig. 1a of the main text), which is quantitatively proven by Geometrical Phase Analysis (GPA) S6. The atomic stacking is in good agreement with the expected (002) growth. Notice that the Ge-Ge dumbbells are perfectly visible showing a perfect diamond structure. The power spectrum or fast Fourier transform (FFT) obtained on the atomic resolution HAADF-STEM image, shown in the bottom, gives us information on the frequency (reciprocal) space, nearly equivalent to a diffraction pattern, which confirms the planes and directions directly observed in the image. b) Triple-axis $\omega$–$2\theta$ scan through Si(004) and dynamical simulation. The inset shows the simulated QW profile, designed to match the profile found by TEM (Fig. 1a of the main text) and from EELS (Fig. S5).

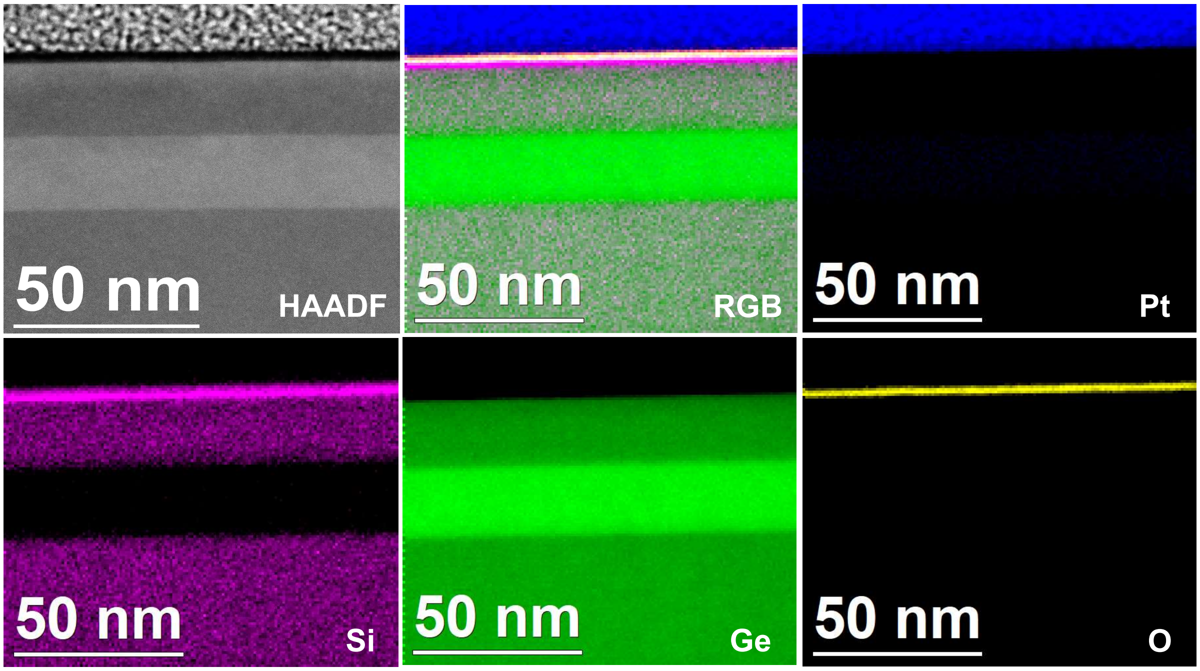


Figure S4: Qualitative composition distribution of the heterostructure, obtained by core-loss electron energy-loss spectroscopy (EELS), showing that the quantum well is close to be pure germanium. This is confirmed by the quantitative analysis shown in Fig. S5. The EELS maps were taken at 200 kV, with a spatial resolution of 1 nm.

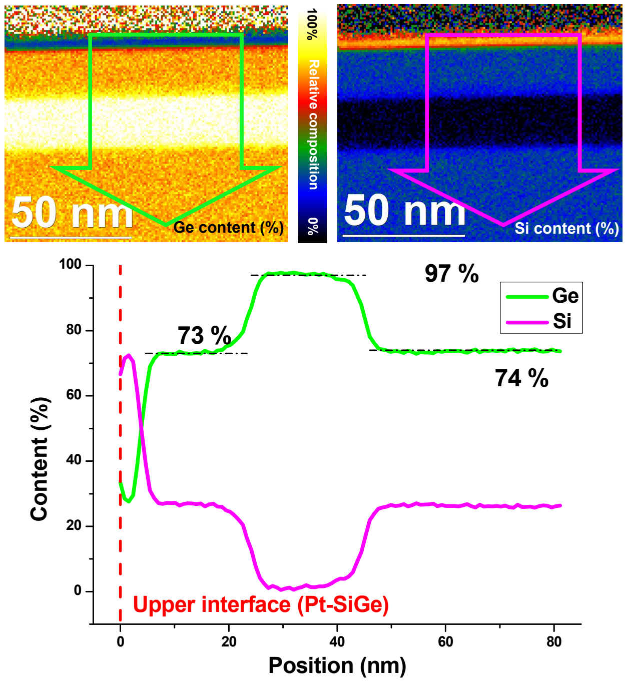


Figure S5: Quantitative composition distribution of both germanium and silicon content in the quantum well and its surrounding layers, obtained by core-loss electron energy-loss spectroscopy (EELS). In order to get the displayed stoichiometry and profile, the reference stoichiometry was taken from the substrate, given by the X-Ray Diffraction measurements on it, which is proven to be constant along its extension. The profile follows the orientation defined by the arrows in the colour maps. The profile is taken from top to bottom, starting at the platinum protection area. The average values shown, and therefore, the stoichiometry, have an experimental uncertainty of 3%. The EELS maps were taken at 200 kV, with a spatial resolution of 1 nm.

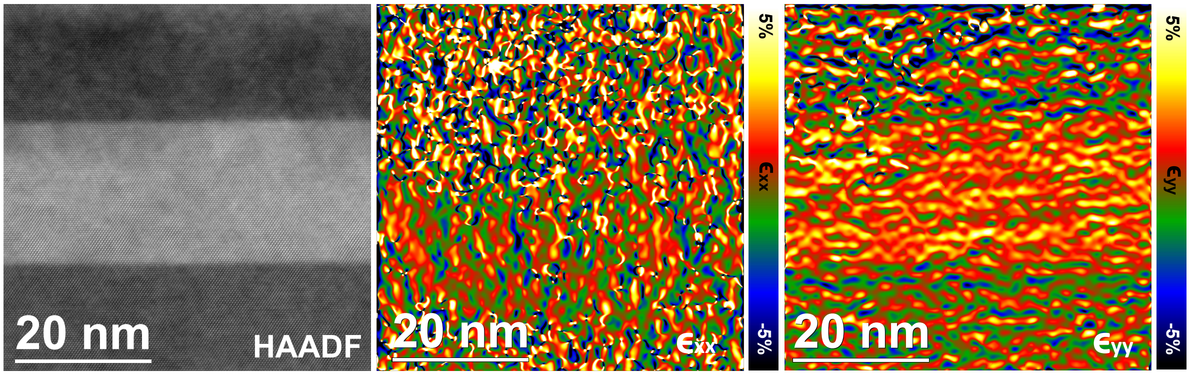


Figure S6: Geometrical Phase Analysis (GPA) applied to the left HAADF-STEM image and the resulting map of the diagonal components of the strain tensor. The reference for the relaxed material is the substrate. $\epsilon xx$ displays the information relative to the strain of the vertical planes ($\bar{2}20$), where the average mismatch of the quantum well with respect to the reference (substrate) is 0.03%, which, given the found composition, is translated into a compressive strain of -0.96% of these vertical planes. $\epsilon yy$ displays the information relative to the strain of the horizontal planes (002), where the average mismatch of the quantum well with respect to the reference (substrate) is 1.27%, which, given the found composition, is translated into a tensile strain of 0.27% of these horizontal planes. Regarding these values, we can conclude that the epitaxy and the matching of the quantum well and the substrate is totally free of plastic relaxation, and with full elastic strain.

# 4 Device characterization

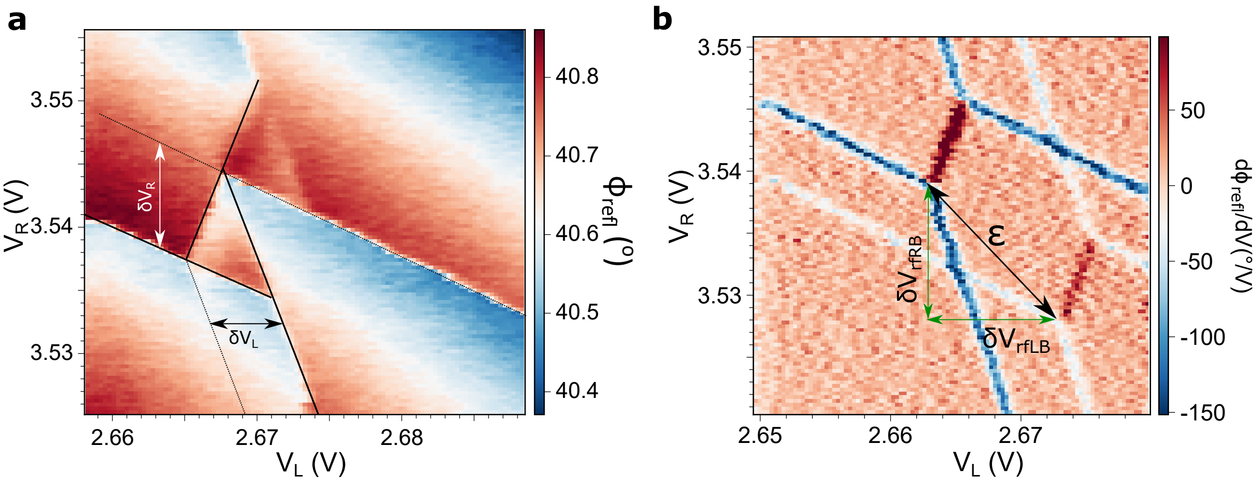


Figure S7: a) Bias triangles acquired with 500 μeV bias. $\delta V_L = 5\,\text{mV}$ and $\delta V_R = 8\,\text{mV}$ leading to the lever arms[6] $\alpha_L \approx 0.10\,\text{eV/V}$ and $\alpha_R \approx 0.06\,\text{eV/V}$. b) Derivative of reflected phase as a function of plunger gate voltages. During acquisition a pulse of $Amp = 1.3\,\text{V}$ was applied to gates LB ($-Amp$) and RB ($+Amp$) for 25% of the duty cycle while 75% of it had no pulse applied. As a consequence the stability diagram shifts diagonally and doubles since the data acquisition averages over both charge configurations. The diagonal black arrow is equivalent to the detuning axis and connects two corresponding triple points. This allows us to extract the rf lever arms for the gates LB and RB: $\delta V_{rfLB} = 11.1\,\text{mV}$, $\delta V_{rfRB} = 9.8\,\text{mV}$, $\alpha_{rfLB} = \frac{\delta V_{rfLB}}{Amp}\alpha_L \approx 854\,\mu\text{eV/V}$ and $\alpha_{rfLB} = \frac{\delta V_{rfRB}}{Amp}\alpha_R \approx 454\,\mu\text{eV/V}$. The maximum pulse amplitude we can apply is 5 V on each barrier gate corresponding to a maximum detuning $\epsilon_{max} = 5\sqrt{\alpha_{rfLB}^2 + \alpha_{rfRB}^2} \approx 4.8\,\text{meV}$.

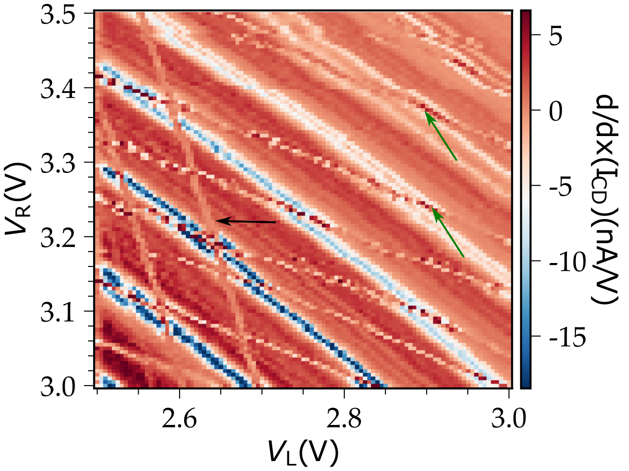


Figure S8: Stability diagram recorded from the current through the charge sensor and differentiated. The black arrow points to the last observable transition in the left dot, allowing precise determination of the hole number in this dot. Green arrows highlight two transitions of the right dot. We are not able to completely deplete the right dot such that a determination of the hole number is not possible here.

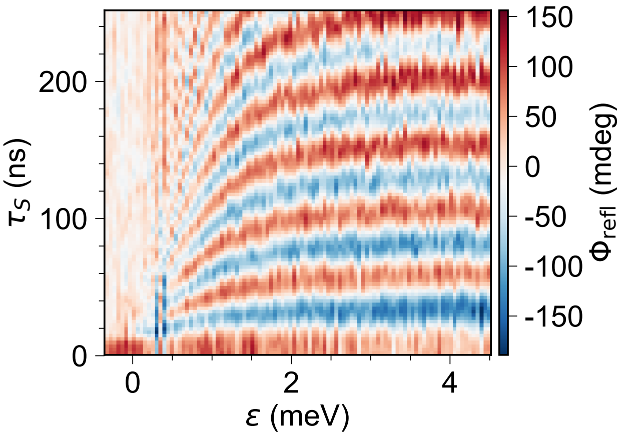


Figure S9: Exchange oscillations for $V_{CB} = 950\,\mathrm{mV}$ at $1\,\mathrm{mT}$. Here the tunnel coupling is tuned to a very small value by CB. Hence, $J$ is reduced and $\Delta g \mu_B B$ dominates at very high values of detuning. From 2 to $4.5\,\mathrm{meV}$ detuning we observe no big change in the oscillation period. Therefore, we assume $\frac{\delta \Delta g}{\delta \epsilon} \to 0$ and justify the form of equation (2) of the main text.

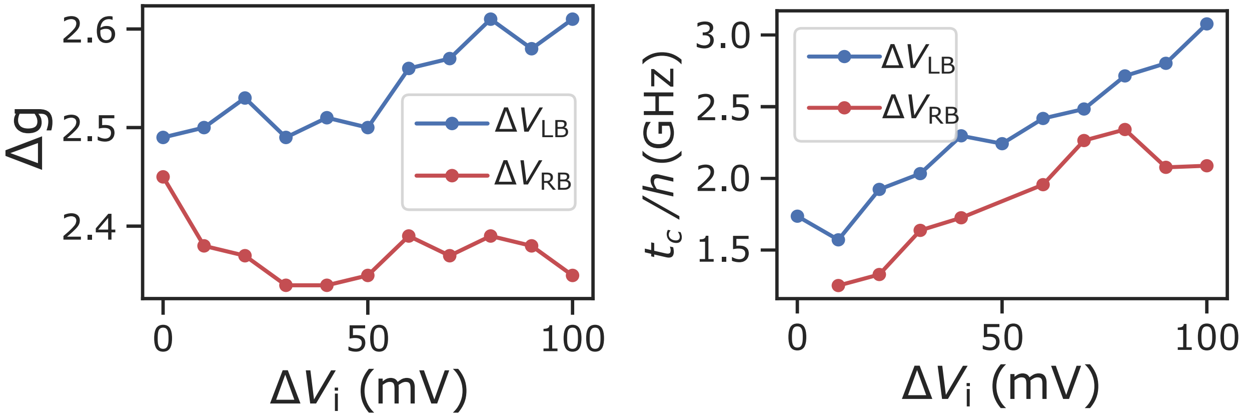


Figure S10: Left: $\Delta g$ as a function of the voltages on LB (blue) and RB (red). Compared to Fig. 3g of the main text here we only see a change of 0.1 in the $g$-factor difference over a range of $100\,\mathrm{mV}$ for both gates. Right: $t_C$ as a function of the voltages on LB (blue) and RB (red). The tunnel coupling can be changed by more than $1\,\mathrm{GHz}$ by applying $100\,\mathrm{mV}$ more on LB. Although the influence of LB and RB on the tunnel coupling is not as large as CB (see Fig. 4h of the main text) the combination with the $g$-factor dependences for these two gates allows to tune $t_C$ and $\Delta g$ almost independently. This ultimately enables precise control over the potential landscape of the dots facilitating the search for noise sweet spots (see discussion of equation (2) of the main text).

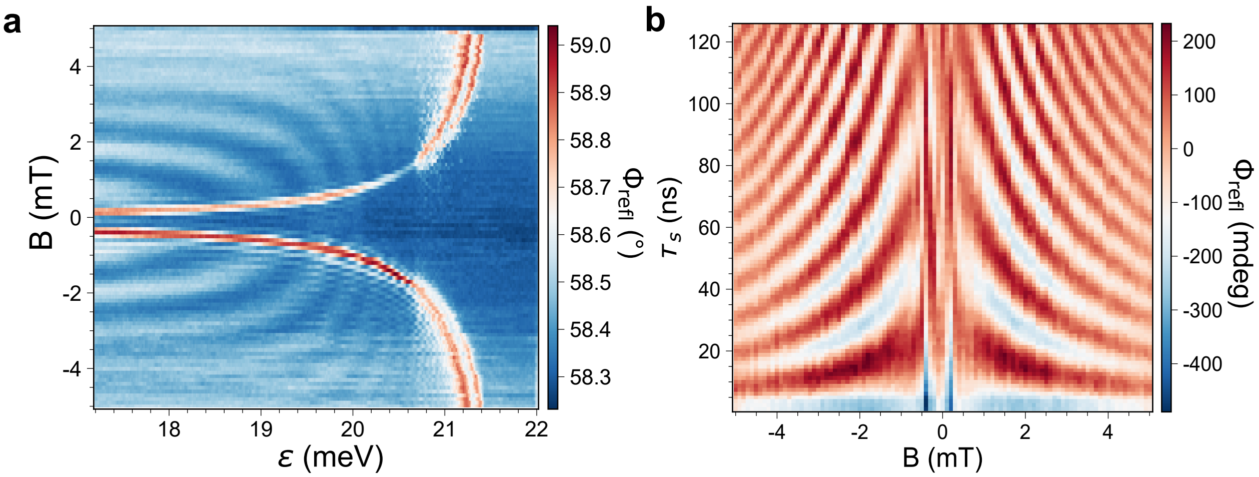


Figure S11: a) Spin-funnel acquired at the transition $(3, 2n+1) \leftrightarrow (2, 2n+2)$ (equivalent to $(1, 1) \leftrightarrow (0, 2)$) with the measurement point fixed at $\epsilon = 22\,\mathrm{meV}$ and same center barrier voltage as in Fig. 2e of the main text. b) X-oscillations at the transition in a) at $\epsilon = 17.2\,\mathrm{meV}$. The rotation frequency is slightly lower than in Fig. 3c of the main text and we extract $\Delta g = 1.4$.

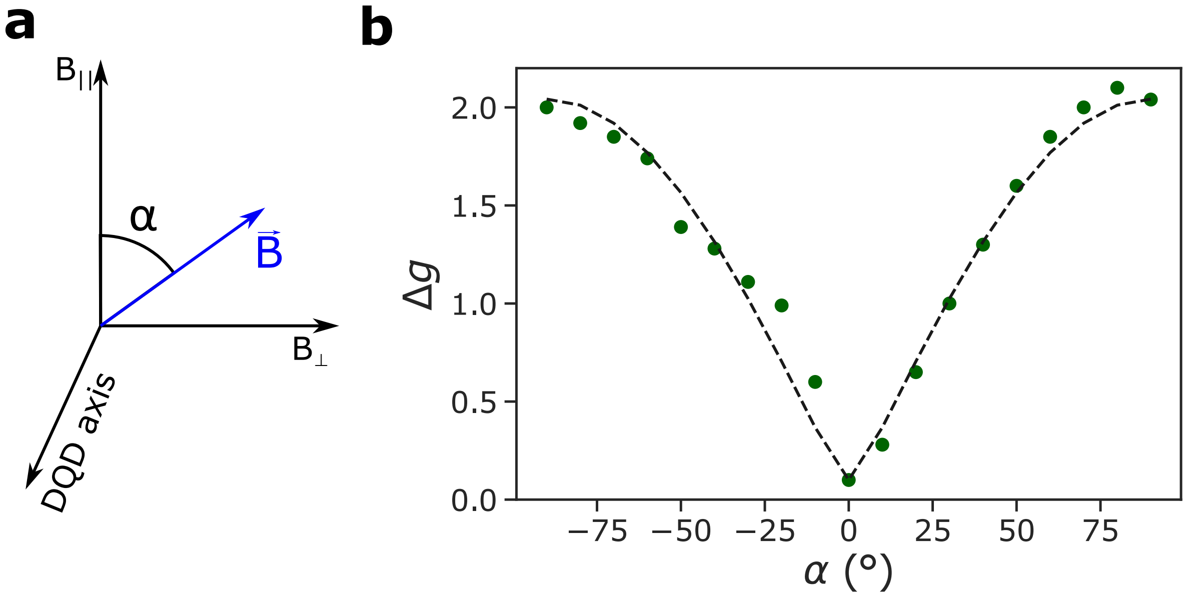


Figure S12: a) Direction of the applied magnetic field with respect to the DQD axis. The main paper focuses on $B_\perp$. Here the angle $\alpha$ is tilted and $\Delta g$ is measured. b) $\Delta g$ as a function of $\alpha$. A clear anisotropy can be observed and the black dashed line is a fit to $\Delta g = \sqrt{(\Delta g_\perp \sin\alpha)^2 + (\Delta g_\parallel \cos\alpha)^2}$, with $g_\perp = 2.04$ and $g_\parallel = 0.11$.

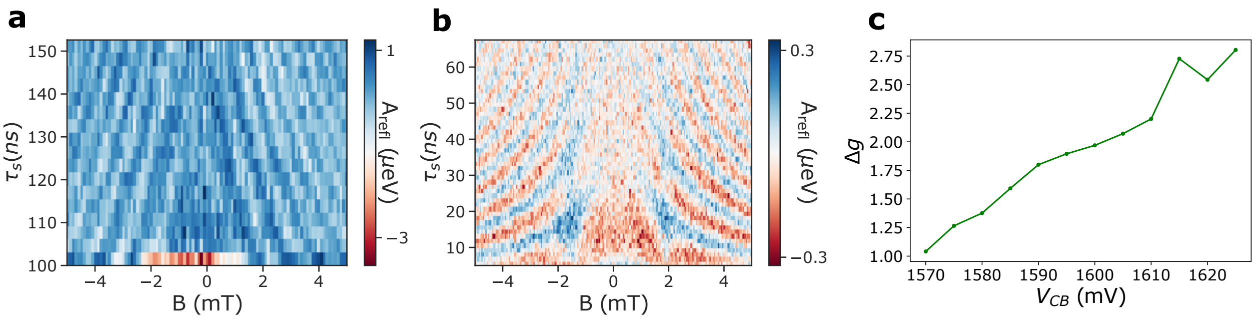


Figure S13: a) $S-T_0$ oscillations in a second device. The g-factor difference we extract from this plot is 1.8. b) $S-T_0$ oscillations in a third device. c) From oscillations at different center barrier voltage we extract the $\Delta g$ dependence on $V_{CB}$. We find an opposite trend to the one observed in Fig.3g: now $\Delta g$ increases with $V_{CB}$. Nevertheless, the reproducibly large and tunable $\Delta g$ make Ge singlet-triplet qubits an interesting candidate for qubit integration.

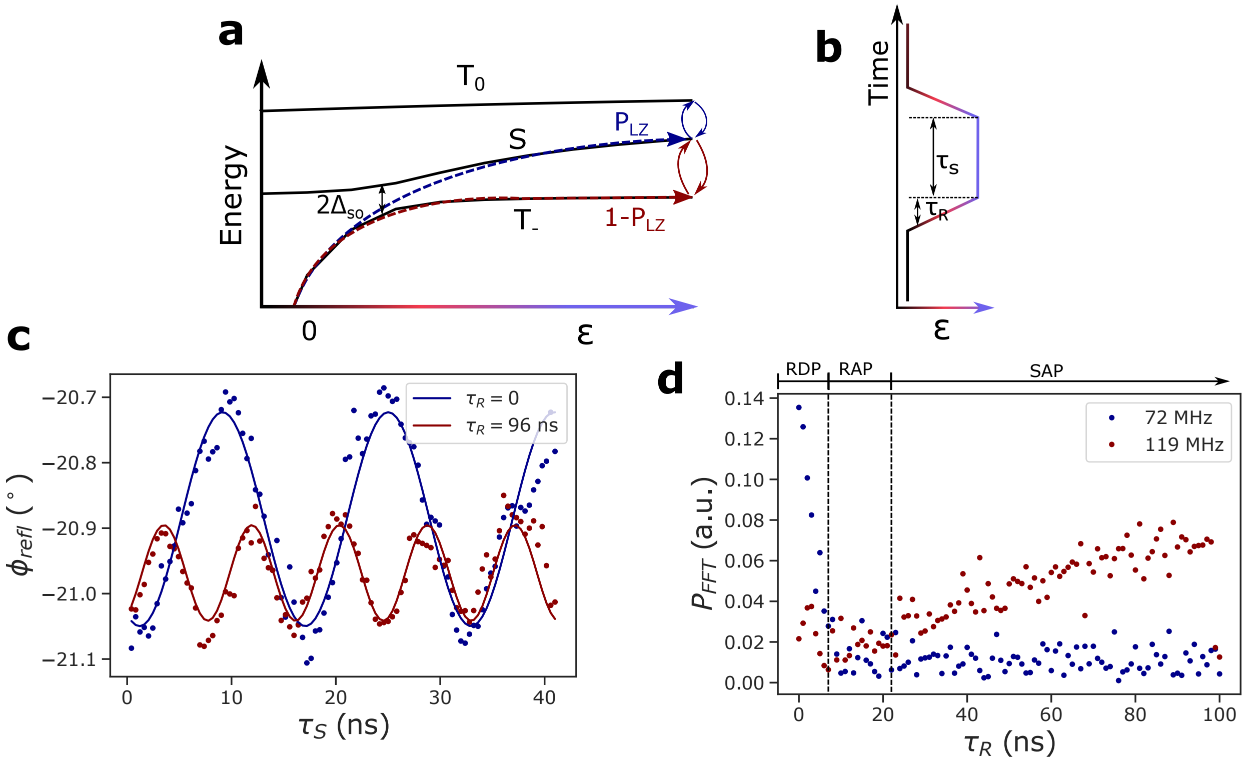


Figure S14: a) Dispersion relation close to the $S - T_-$ avoided crossing. The size of the anticrossing is determined by $\Delta_{SO} = t_{SO} sin(\Omega/2)$, where $\Omega$ is the mixing angle. A fast pulse from low $\epsilon$ (left) to high $\epsilon$ (right) causes the system to remain in the singlet state (blue trajectory). A slow pulse will cause the system to remain in the ground, which at high $\epsilon$ is $T_-$. The probability of maintaining a singlet or evolving to a triplet is determined by the Landau-Zener probability $P_{LZ} = \exp\left\{\frac{2\pi\Delta_{SO}^2}{\hbar v}\right\}$, with $v = \frac{dE}{dt} = \frac{dE}{d\epsilon}\frac{d\epsilon}{dt}$ being the velocity (how fast the energies are changed, e.g. how fast $\epsilon$ is ramped), $dE = |E_Z^T/2 - J|$ is the energy difference between $T_-$ and $S$ and $\frac{d\epsilon}{dt}$ is the ramp rate. b) Pulse sequence to discriminate $S - T_0$ and $S - T_-$ oscillations. After initializing in singlet in (2,0) the system is ramped to (1,1) in a ramp time $\tau_R$. After a separation time $\tau_S$ the system is ramped to (2,0) again at the same ramp speed. The resulting oscillations are depicted in c). c) $S - T_0$ oscillations (blue) are evident when the system is pulsed over the anticrossing quickly ($\tau_R = 0$, we note, however, that the AWG has a nominal rise time of 1.1 ns). $S - T_-$ oscillations (red) emerge when the ramp time is longer and $S - T_-$ mixing occurs. The amplitude of these oscillations depends on $\tau_R$ as confirmed by the Fourier amplitude in d). d) Power of the Fourier transform as a function of ramp time for the $S - T_0$ (blue) and $S - T_-$ (red) oscillation frequency. For ramp times smaller than 10 ns the $S - T_0$ frequency dominates, in line with the observations in c). The slower the ramp the more the $S - T_-$ frequency becomes prominent because the slow passage over the anticrossing mixes $S$ with $T_-$. In fact, the speed of a pulse on $\epsilon$ will lead to 3 different regimes: the rapid diabatic passage (RDP), the rapid adiabatic passage (RAP) and the slow adiabatic passage (SAP). The passage with respect to the charge anticrossing determined by $t_C$ is always adiabatic. In RDP the system passes rapidly over the $S - T_-$ anticrossing and the state remains a singlet also at high detuning. This happens for $\tau_R < 10$ ns. In RAP the passage over the anticrossing is still diabatic but the ramprate is now slow enough to allow the singlet to evolve to $\uparrow\downarrow$ at high detuning. This means that the system is in an eigenstate state of the Hamiltonian and no oscillations will be observed ($10\,\text{ns} < \tau_R < 40\,\text{ns}$). Gradually increasing $\tau_R$ will make the passage over the anticrossing more and more adiabatic (SAP). Now $S - T_-$ mixing causes oscillations to appear at a frequency $f = \frac{\Sigma g\mu_B B/2 - J}{h}$ with an amplitude that still depends on $\tau_R$ and, therefore, the degree of mixing.

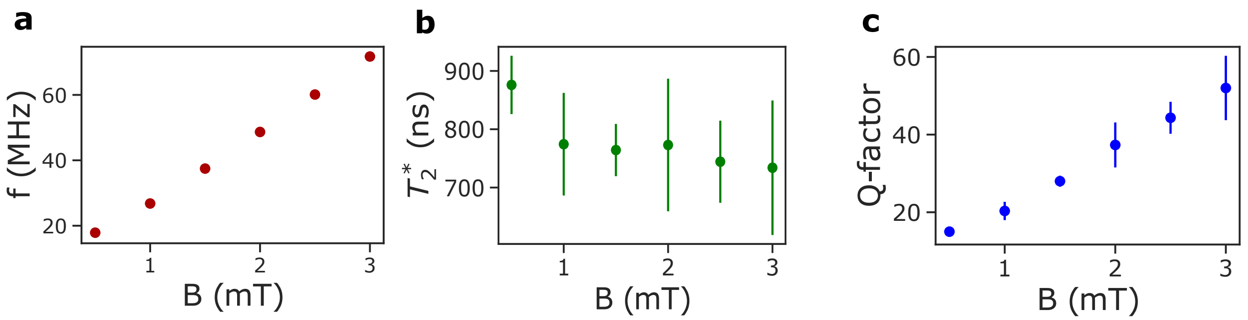


Figure S15: Frequency, $T_2^*$ and Q-factor reported for a different gate configuration than in the main text averaged over 3 measurements taken at different time points over the course of 3 days. a) Frequency as a function of magnetic field strength. b) $T_2^*$ as a function of $B$. We observe a slight decrease of $T_2^*$ with magnetic field. The errors correspond to one standard deviation. For field values bigger than 2 mT the errors are larger as a result of a smaller oscillation amplitude and correspondingly worse fitting conditions. c) $Q = f \times T_2^*$ as extracted from a) and b). A linear increase of $Q$ with $B$ becomes evident. This means that it is possible to enhance the quality of the qubit by increasing the $S - T_0$ oscillation frequency, without affecting the dephasing time too negatively. At 3 mT we extract a $Q$-factor of 52.

## 4.1 Calibrating the refocusing pulse

Spin echo techniques like Hahn echo and Carr-Purcell-Meiboom-Gill (CPMG) are easily implemented when two perpendicular rotation axis are available. The singlet-triplet qubit, however, comes with the constraint of $J(\epsilon) > 0$ for every $\epsilon$, and $\Delta g \mu_B B \neq 0$. This means that the rotation angle $\theta = \arctan(\frac{\Delta g \mu_B B}{J(\epsilon)})$ can neither be 0 nor 90 degrees. This leads to complications when trying to perform the known echo techniques. Here we implement a spin echo by applying a refocusing pulse calibrated to a specific initial and final state. We let the system evolve freely at large detuning ($\epsilon_f$), on the trajectory depicted in Fig. 3a of the main text and Fig. S16c. The initial state for the refocusing pulse is $|\Psi_i\rangle = \exp(-iH(\epsilon_f)\tau_S/\hbar)\,|\Psi_0\rangle$, where $H(\epsilon_f)$ is the hamiltonian defined in equation 1 of the main text with $\epsilon_f = 4.5\,\text{meV}$, and $\Psi_0 = S$. The evolution time $\tau_S$ is chosen as $(2n + 1/2)t_\pi$ where $t_\pi$ is the time needed for a $\pi$-rotation at $\epsilon_f$. The refocusing pulse is calibrated to obtain the final state $|\Psi_1\rangle = \exp(-iH(\epsilon_f)(\tau_S + t_\pi)/\hbar)\,|\Psi_0\rangle$. Then the system is left to evolve freely again for a time $\tau_S + \delta t$ at $\epsilon_f$. The total evolution time $\Sigma\tau_S = 2(2n + 1/2)t_\pi + \delta t$ leads to a minimum in $\text{P}_\text{S}$ at $\delta t = 0$ if no refocusing pulse has been applied, and to a maximum in $\text{P}_\text{S}$ at $\delta t = 0$ if a correct refocusing pulse has been applied. In Fig. S16 we demonstrate a bad (a)) and a good (b)) calibration of $\tau_S$ and the refocusing pulse and illustrate the respective state evolution on the Bloch sphere in Fig. S16c-e. In a) the blue curve is obtained with no refocusing pulse. The state evolves on the trajectory in Fig. S16c. At $\delta t = 0$ we would expect to find a small singlet probability. However, we observe a maximum in the singlet probability suggesting that the total free evolution time is $(4n + 2)t_\pi$ instead of $(4n + 1)t_\pi$. The red dots correspond to the trace obtained from the same free evolution time but with a refocusing pulse applied. The state evolution is depicted in Fig. S16d. We observe a change in the oscillation amplitude and average value. This indicates that after the refocusing pulse, the state is not evolving on the same trajectory as before the pulse. The red trajectory on the Bloch sphere shows that a higher triplet probability is expected than for the blue trajectory because the refocusing pulse is not applied at the correct time. In b) we adjusted the free evolution time to obtain a high triplet probability after $\Sigma\tau_S$ without refocusing pulse (blue). The refocusing pulse is now calibrated to obtain a singlet state at $\delta t = 0$ (red). The state evolution on the Bloch sphere in Fig. S16e shows that the red and blue trajectory coincide meaning that the refocusing pulse is applied at the right time and has the correct length. With this calibration we can perform the echo sequences and extract the decay times displayed in Fig. 5d of the main text.

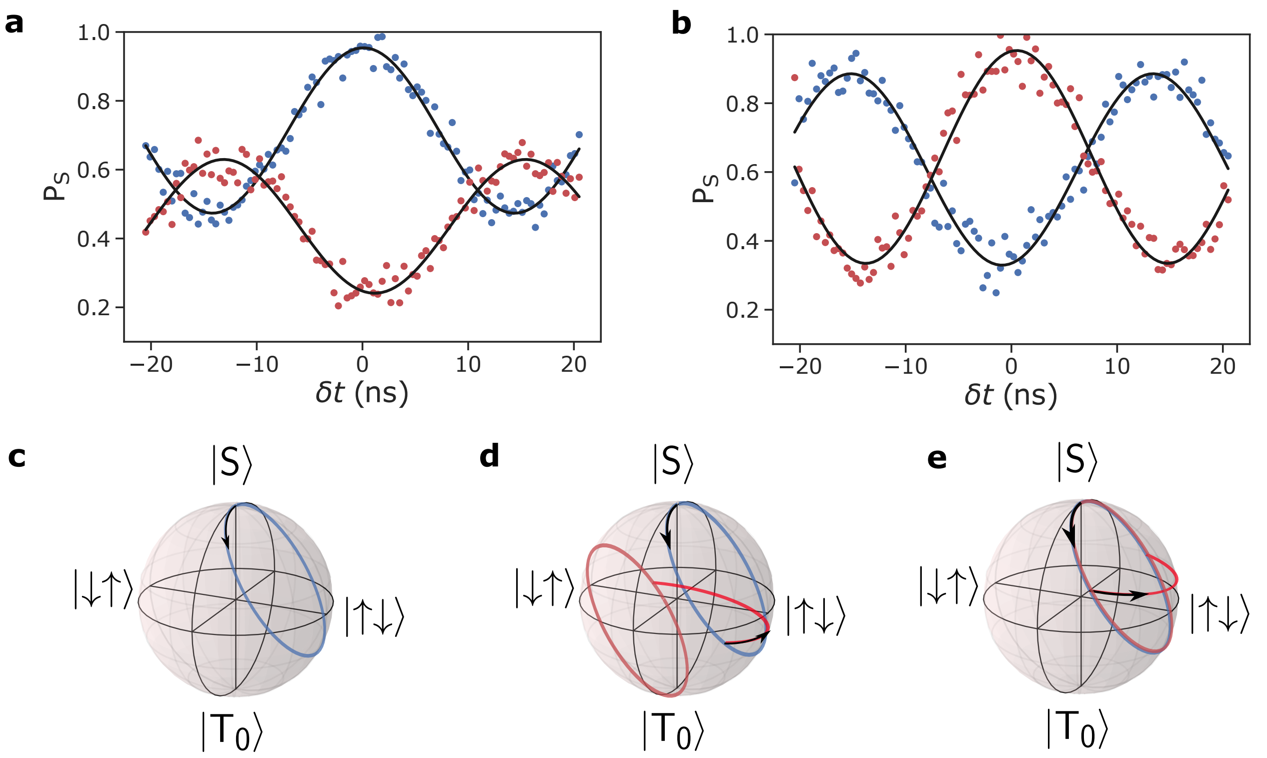


Figure S16: Echo oscillations as a function of $\delta t$ for no (blue) or one (red) recovery pulse. The aim is to generate an echo sequence that recovers the singlet state at the end of a sequence. Because of the tilted oscillation angle during free evolution at high detuning and also during exchange pulses the typical Hahn echo sequence cannot be applied. We, therefore, need to calibrate the exchange pulse but also the free evolution time. We choose $\tau_S = (2n + 1/2)t_{\pi_x}$. We either apply no exchange pulse after $\tau_S$ or apply one. Then we let the system evolve again for a time $\tau_S \pm \delta t$. For the sequence with no exchange pulse applied we expect that for $\delta t = 0$ the system will be at the minimum singlet probability. The exchange pulse, on the other hand, should add a phase of $\pi$ to the state such that we recover the maximum singlet probability at the end of the sequence for $\delta t = 0$. a) Blue dots correspond to $\Sigma\tau_S = 580\,\mathrm{ns}$ without exchange pulse and red dots are with an exchange pulse of 4.5 ns at $\epsilon_r = 0.72\,\mathrm{meV}$. We obtain a maximum at $\delta t = 0$ for the blue curve meaning that $2\tau_S \neq (2n + 1/2)t_{\pi_X}$. The red curve on the other hand shows that, while we obtain a phase shift of $\approx \pi$ with respect to the blue curve, the average singlet probability is smaller (see Fig. S16d ). This means that we over rotated the state during exchange. Both $\tau_S$ and the exchange pulse need further calibration. b) Calibrated pulses. Blue dots correspond to $\Sigma\tau_S = 600\,\mathrm{ns}$ and no refocusing pulse has been applied. Red dots are also $\Sigma\tau_S = 600\,\mathrm{ns}$ but exactly in between a refocusing pulse of 4.5 ns at $\epsilon_r = 0.64\,\mathrm{meV}$ was applied corresponding to a phase shift of $\pi$ and a consequent maximum at $\delta t = 0$. This indicates that the singlet has been recovered. c) State evolution on the Bloch sphere at $\epsilon_f$. d) State evolution on the Bloch sphere at $\epsilon_f$ with a refocusing pulse applied at $\epsilon_r = 0.72\,\mathrm{meV}$. Because the refocusing pulse is applied at the wrong time the trajectory of the state after the recovery (red) evolves in a different plane than before recovery. This leads to an increased triplet probability. e) State evolution on the Bloch sphere at $\epsilon_f$ with a refocusing pulse applied at $\epsilon_r = 0.64\,\mathrm{meV}$. Here the refocusing pulse is applied at the correct time and the refocused trajectory coincides with the initial trajectory. In this way spin-echo can be performed.

## 4.2 Pulsing and $T_1$

During the acquisition of Fig. 2a,b,e, Fig. 3c and Fig. 4c of the main text the signal was integrated over 100 ms for each data point under continuous pulsing (Fig. S17 Left). The time spent in the measurement point $t_M \gg \tau_s$ meaning that the largest portion of the signal is actually taken at the M point. Figures 3f, 4f, 4g and 5e of the main text on the other hand are obtained by averaging 500 single shot measurements. The signal is integrated from the moment the system is returned to the measurement point. Before the next pulse starts, the system is left for 100 µs at the measurement point and the average signal $\Phi_{\text{offset}}$ (see Fig. S18a) is substracted from the previously integrated signal to account for fluctuations in the charge sensor. The phase signal is then transformed to probability by considering the signal difference between (1,1) and (2,0) $\delta\Phi_{\text{refl}}$. $\text{P}_\text{S} = 1 - \frac{\Phi_{\text{refl}} - \Phi_{\text{offset}}}{\delta\Phi_{\text{refl}}}$. The signal to noise ratio did not allow us to distinguish singlet and triplet states in single shot measurements, only after averaging the distinction becomes clear.

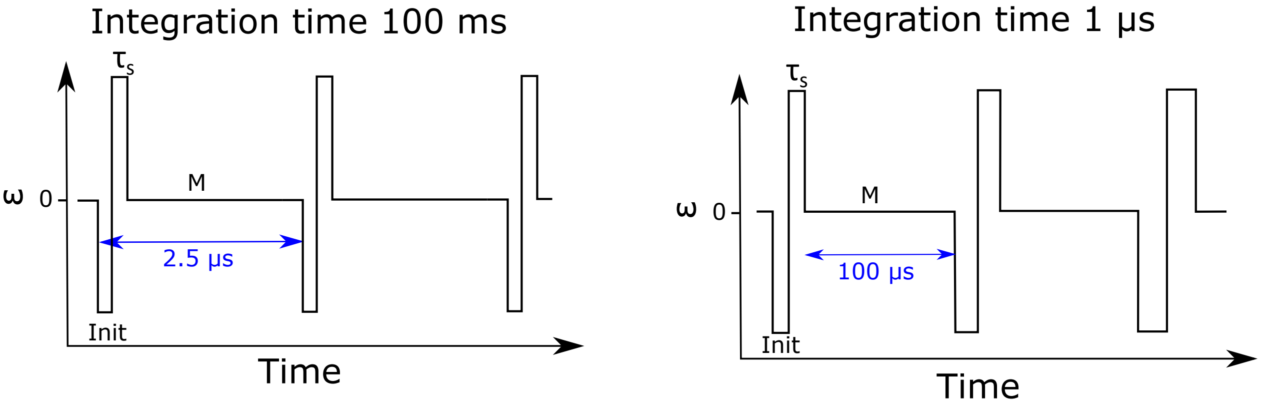


Figure S17: Left: Continuous pulsing. The integration time is 100 ms and the same pulse is repeated 4000 times. Since most of the duty cycle is spent in the measurement point M, the resulting signal can be interpreted as the signal in the measurement point. The intialization (Init) pulse has the same amplitude but opposite sign as the separation pulse and the same length $\tau_S$. This ensures that there is no DC offset on the pulse. Right: averaged single shot. The integration time is 1 µs. The separation time is stepped for consecutive pulses and only the signal in the measurement point is considered (see Fig. S18). During the whole pulse train the data is recorded and averaged 500 times. The singlet and triplet probabilities are then extracted in post-processing.

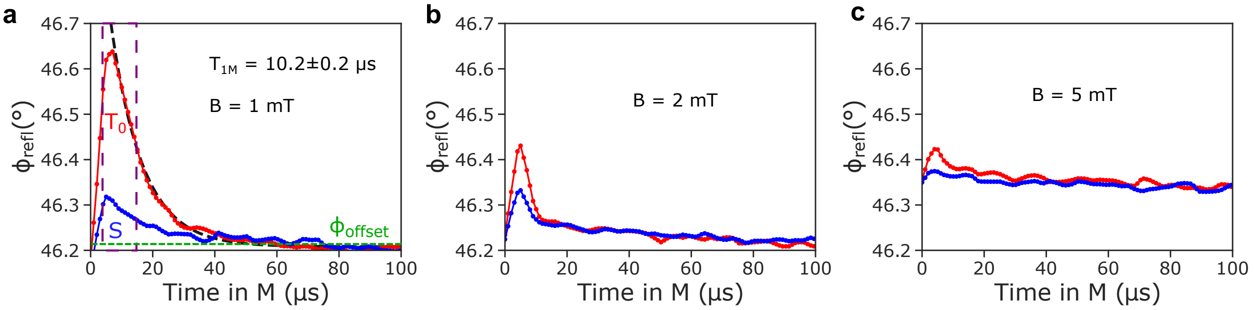


Figure S18: $T_1$ in the measurement point at different magnetic field. a) Averaged single shot traces of a singlet (blue) and a $T_0$ (red) state as a function of time in the measurement point. The black dashed line is a fit to $A\exp\left(\frac{-(t-t_0)}{T1}\right) + C$. At 1 mT we extract $T_1 = 10.2 \pm 0.2$µs. The signal inside the dashed region is averaged giving the difference between the $T_0$ and the $S$ state. $\phi_{\text{offset}}$ (green) is substracted from the signal to account for drifts in the charge sensor signal over time. b) At 2 mT the amplitude of the triplet signal is greatly reduced as a consequence of decay from $T_0$ to $S$ during measurement. c) At 5 mT $S$ and $T_0$ states become almost indistinguishable.

## 5 $T_2^*$ extraction for $V_{CB}$ and $\epsilon$ dependence

The inhomogeneous dephasing time ($T_2^*$) is extracted from fits to X-rotations and Z-rotations. We find that generally a gaussian decay can be observed ($\exp(-(t/T_2^*)^2)$). Fig. S19 displays the traces used to determine the values of Fig. 3h of the main text. Figures S20,S21 and S22 display Z-rotations at different detuning values. The coherence times extracted here are depicted in Fig. 4i of the main text.

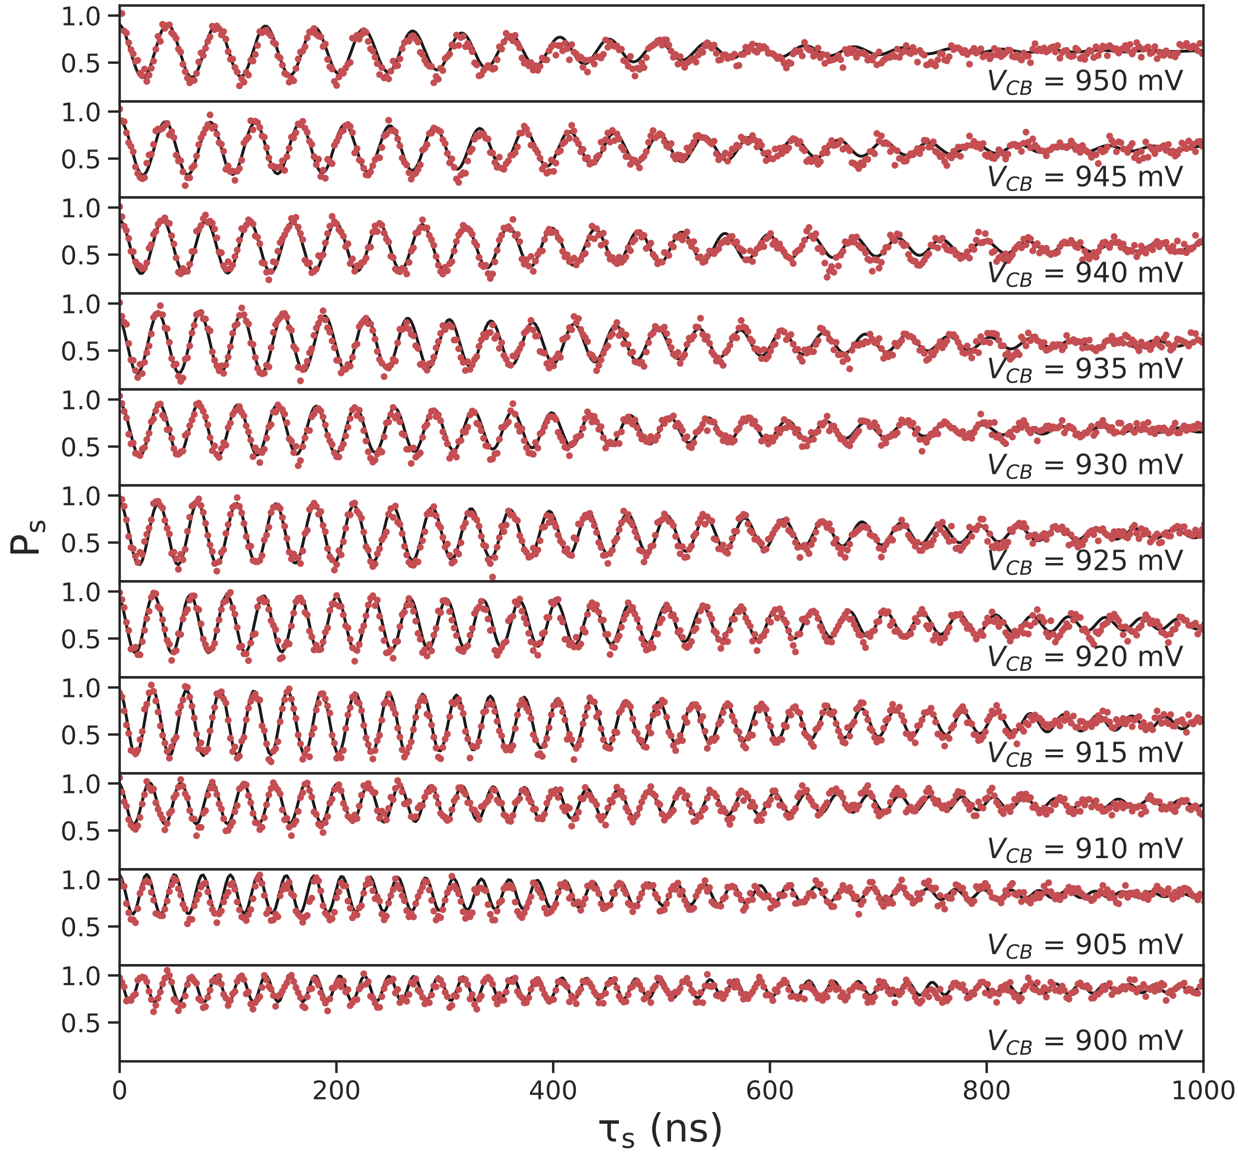


Figure S19: X-rotations. $P_S$ as a function of $\tau_S$ at $B = 1\,\text{mT}$ and $\epsilon = 2.8\text{meV}$ for the center barrier voltages reported in the inset. Black lines are fit to $P_S = A\cos(2\pi f + \phi)\exp\left(-(t/T_2^*)^2\right) + C$. The extracted $T_2^*$ is reported in the main text (Fig. 3h).

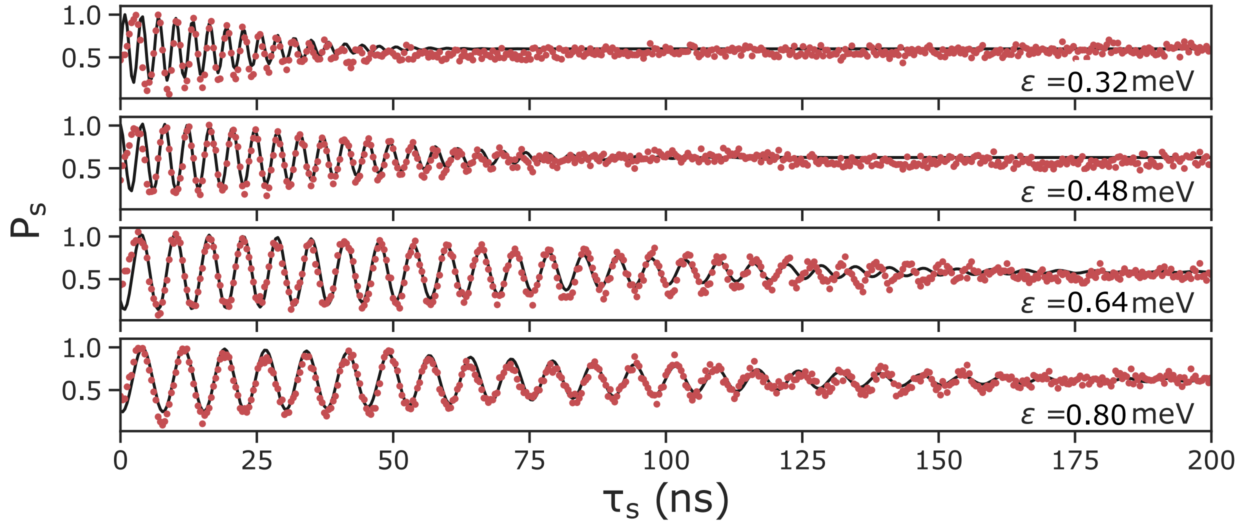


Figure S20: Z-rotations. $P_S$ as a function of $\tau_S$ at $B = 1\,\mathrm{mT}$ and $V_{CB} = 910\,\mathrm{mV}$ for low detuning. The extracted $T_2^*$ is reported in the main text (Fig. 4i)

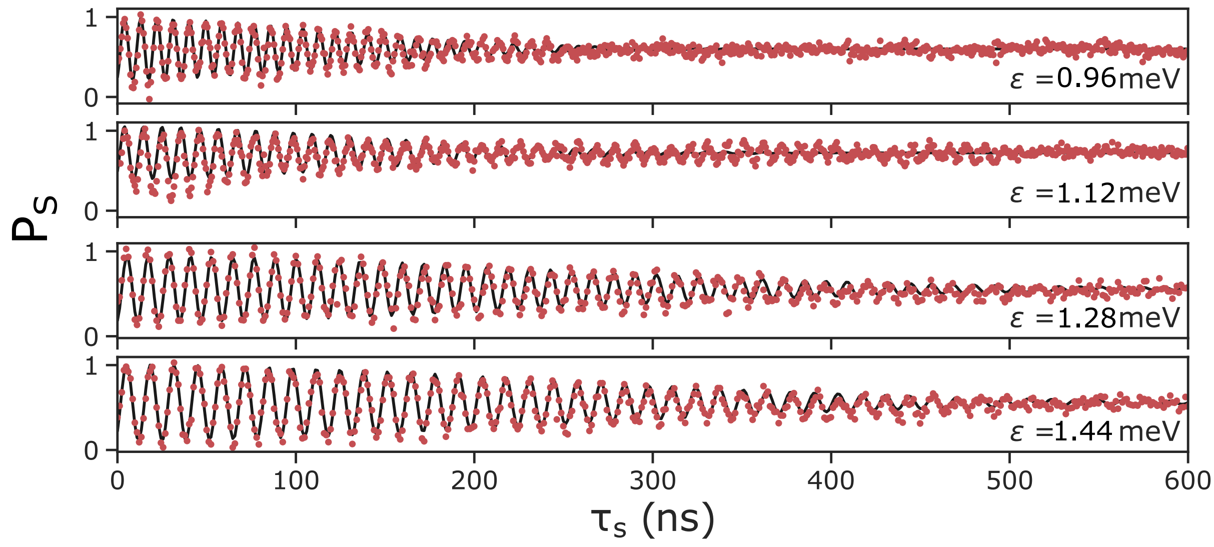


Figure S21: Z-rotations. $P_S$ as a function of $\tau_S$ at $B = 1\,\mathrm{mT}$ and $V_{CB} = 910\,\mathrm{mV}$ for medium detuning.The extracted $T_2^*$ is reported in the main text (Fig. 4i)

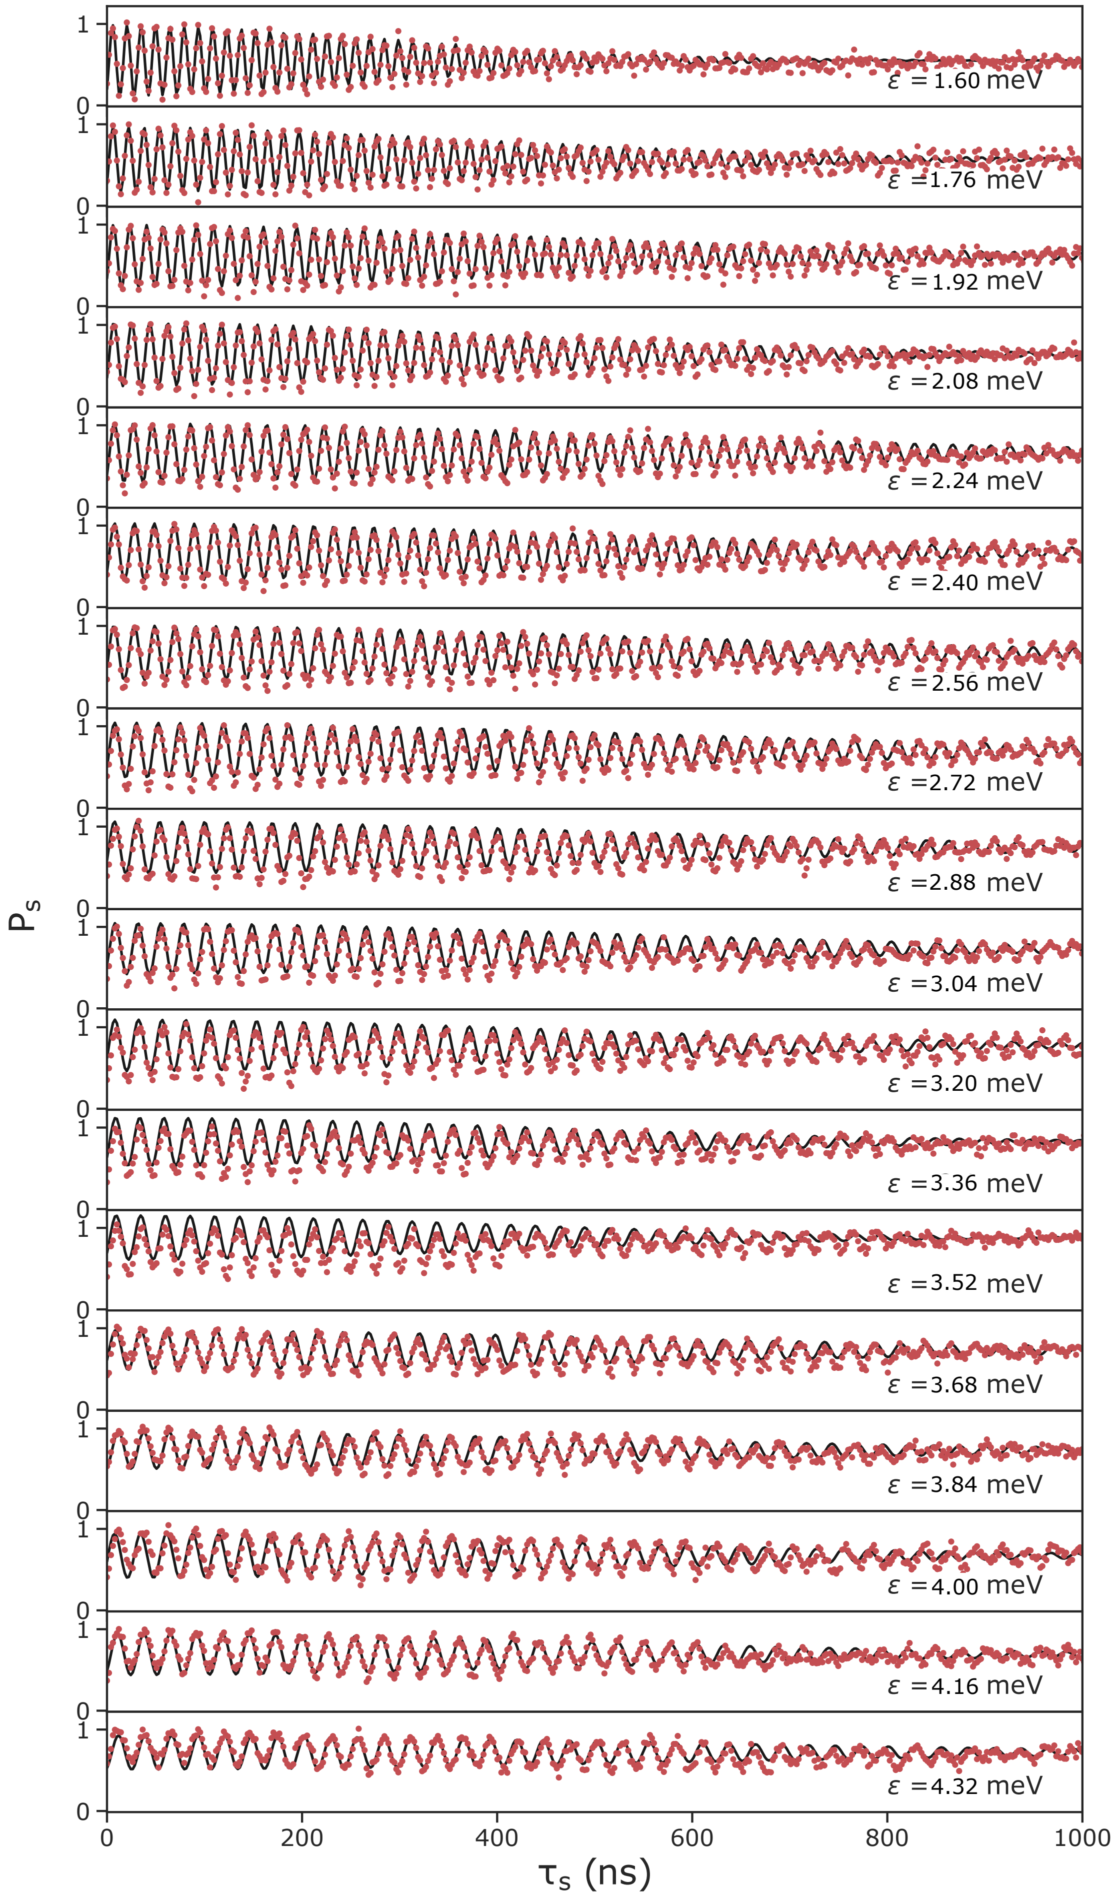


Figure S22: Z-rotations. $P_S$ as a function of $\tau_S$ at $B = 1\,\mathrm{mT}$ and $V_{CB} = 910\,\mathrm{mV}$ for high detuning. The extracted $T_2^*$ is reported in the main text (Fig. 4i).

# References


[1] Froning, F. N. M. *et al.* Strong spin-orbit interaction and $g$-factor renormalization of hole spins in Ge/Si nanowire quantum dots. *arXiv: 2007.04308 [cond-mat]* (2020).

[2] Mutter, P. M. & Burkard, G. g-tensor resonance in double quantum dots with site-dependent g-tensors. *Materials for Quantum Technology* (2020).

[3] Hÿtch, M., Snoeck, E. & Kilaas, R. Quantitative measurement of displacement and strain fields from HREM micrographs. *Ultramicroscopy* **74**, 131–146 (1998).

[4] de la Mata, M., Magén, C., Caroff, P. & Arbiol, J. Atomic scale strain relaxation in axial semiconductor III–V nanowire heterostructures. *Nano Letters* **14**, 6614–6620 (2014).

[5] Kriegner, D., Wintersberger, E. & Stangl, J. xrayutilities: a versatile tool for reciprocal space conversion of scattering data recorded with linear and area detectors. *Journal of Applied Crystallography* **46**, 1162–1170 (2013).

[6] van der Wiel, W. G. *et al.* Electron transport through double quantum dots. *Reviews of Modern Physics* **75**, 1–22 (2002).
